# Supplementary material for: lepton number survival in the cosmic neutrino background
Source: arXiv:2212.01038 source file (2022-12-02)
Supplement: Supplementary file 1 [file appendix.tex]

\appendix
\section{Press-Schechter formalism}
\label{app:PS}
We present here some details of the formalism used to compute N as well as some justifications for the choice of parameters. For the sake of clarity, we recall our master formula :
\begin{align}
\label{eq:masterappendix}
	N_{\flip} ={}& \int_0^{z_0}\frac{v(z)dz}{H(z)}\int_{M_{\text{min}}}^{M_{\text{max}}}dM\frac{dn}{dM}\sigma(z,M)\\
	\propto{}& \int dz \frac{(1+z) (1+z)^2}{H_0 \sqrt{\Omega_\Lambda + \Omega_M (1+z)^3}} \int dM
\end{align}
 In the PS formalism, $dn/dM$ is expressed as (see e.g. \cite{gorbunov_introduction_2011}): 
\begin{equation}
\label{eq:dndm}
	\frac{dn}{dM} = -\frac{2\delta_c}{\sqrt{2\pi}\sigma_M^2}\frac{\rho_M}{M^2}\frac{d\sigma_M}{d\mathrm{log}M}\cdot e^{-\frac{\delta_c^2}{2\sigma_M^2}}
%	\label{eq:PS_number_density}
\end{equation}
where the $\delta_c = 1.68$ and the mass variance can be taken from the analytic approximation (see \cite{gorbunov_introduction_2011}) or calculated from the power spectra of inhomogeneties as it is related to distance scale variance $\varsigma_{R} (R)$. Relation is up to variable substitute $R \leftrightarrow M$ from
\begin{equation}
    M = \frac{4}{3}\pi R^3 \rho_{crit} \Omega_M (1+z)^3
\end{equation}
Where $\rho_{crit}$ - critical density of the Universe, $\Omega_M$ - matter fraction of energy density, z - redshift parameter. So mass is related to area with the size R if it was homogeneously filled with matter of $\rho_{crit} \Omega_M (1+z^3)$ density. But this relation is not complete and requires use of growth function (see \cite{dodelson:2003})
\begin{equation}
    D(z) = \frac{5}{2} H(\frac{1}{1+z}, \Omega_M, \Omega_{\Lambda})
\end{equation}
Here H - Hubble parameter, that depends on the redshift z, matter and lambda-term 
So the relation will be:
\begin{equation}
    \sigma_M=\frac{D(1)}{D(z)}\sigma_R \left(^{1/3}\sqrt{\frac{M}{\frac{4 \pi}{3}\rho_{crit}(1+z)^3\Omega_M}}\right)
    \label{eq:sigmaM}
\end{equation}
Coordinate scale variance is calculated from power spectra as:
\begin{equation}
    \sigma^2_R = \int_0^{\inf}{\frac{k^3}{2\pi^2}\mathcal{P}(k)j_1(k R)^2} 
\end{equation}
where $\mathcal{P}(k)$ - power spectrum. $j_1$ - Bessel spherical function.
  Examples of $\sigma_M$ are provided on figure \ref{fig:sigmaRMS}.

\begin{figure}[h]
		\includegraphics[width=\linewidth]{SIgmaM.pdf}
	\caption{$\sigma_M$ as a function of the halo mass for different redshifts.}
	\label{fig:sigmaRMS}
\end{figure}
By plugging (\ref{eq:dndm}) and (\ref{eq:sigmaM}) in (\ref{eq:masterappendix}) and integrating upon the mass, one gets the results displayed on figure \ref{fig:Mdependence} and \ref{fig:Mdependence_speed}.

%\begin{figure}[h]
%		\includegraphics[width=\linewidth]{Mmaxdependence}
%	\caption{$\int dM\frac{dn}{dM}$ as a function of $M_{\text{max}}$ for various $\bmax$. \tcb{legends needed + x axis...}}
%	\label{fig:Mdependence}
%\end{figure}
With such analytic expression we can see, that the dominant contribution for the helicity-flip is given by objects with mass $10^{13} \lesssim M/M_{\odot} \lesssim 10^{14}$ - cross-section depends on the mass of the object with the power low (approximately, since the expression under the logarithm becomes close to zero only for very large masses or small impact parameters), while number of objects with masses $M<10^{14} M_{\odot}$ is $dn/dM \sim M^{-2}$ roughly. Hence, the major mass-dependence cancels-out. Only at the largest masses, when exponential suppression in the number of objects and logarithmic suppression for the cross-section take place, the contribution become smaller, so the $\int \sigma dn/dM $ saturates. The only difference that is left is that the range of integration is highest for large masses and although the integrand is only weakly mass-dependent, the integration range is largest for large masses. 
\begin{figure}[h]
		\includegraphics[width=\linewidth]{sigmadNdMIntegrated}
	\caption{$\int \sigma \cdot dM\frac{dn}{dM}$ as a function of $M_{\text{max}}$ for various neutrino speed. }
	\label{fig:Mdependence_speed}
\end{figure}

It is obvious that any choice of $M_{\text{max}}$ above $10^{15}M_\odot$ is saturating the integrand. This result is valid whatever the neutrinos speed or the choice of maximum impact paramenter.  We stress that the dependence in term of $M_{\text{min}}$ is completely negligible. It was however set to $10^8M_\odot$ which is a reasonable boundary corresponding to really light stellar objects. 

\section{Distribution function}
\label{sec:distr-funct}

The Boltzmann equation in the expanding Universe has the form
\begin{equation}
  \label{eq:2}
  E \frac{\partial f}{\partial t} - H(t) p^2 \frac{\partial f}{\partial E} = I[f]
\end{equation}
If $E^2 = p^2$ then the solution of Eq.~\eqref{eq:2} has the form
\begin{equation}
  \label{eq:3}
  f(p,t) = g\left(\frac{p a(t)}{a_i}\right)
\end{equation}
where function $g(\dots)$ should be chosen such as to put $I[f] = 0$. This is Fermi-Dirac distribution, i.e.\ for fermions Eq.~\eqref{eq:3} is written as
\begin{equation}
  \label{eq:4}
  f(p,t) = \frac 1{\exp(\frac{\sqrt{p^2 a^2(t) + m^2 a_i^2}}{a_i T_i}) + 1} =
  \frac 1{\exp(\frac{\sqrt{p^2 + m^2 a_i^2a^{-2}(t)}}{T(t)}) + 1}
\end{equation}
where $a_i, T_i$ are scale factor and temperature at decoupling (assuming it to be instantaneous and all that) and we introduced
\begin{equation}
  \label{eq:5}
  T(t) \equiv \frac{a_i T_i}{a(t)}
\end{equation}
and
\begin{equation}
  \label{eq:7}
  m \frac{a_i}{a} = m \frac{1+z}{1+z_i}
\end{equation}
Consider time now. $p = m v$ and $T(t) = T_{C\nu B}$. Distribution function has the form
\begin{equation}
  \label{eq:6}
  f(p,t_0) = \frac1{\exp(\frac{mv}{T_{C\nu B}}) + 1}
\end{equation}
as long as $v \gtrsim  \frac{1}{1+z_i}\sim 10^{-10}$
